# Supplementary material for: Recognisable languages over monads
Source: arXiv:1502.04898 source file (2015-02-17)
Supplement: Supplementary file 1 [file appendix-mn.tex]

\section{Proof of the Myhill-Nerode Theorem}
\label{sec:proof-mn}
In this part of the appendix, we prove Theorem~\ref{thm:syntactic-morphism}. The theorem says that for every $\monad$-recognisable language $L \subseteq \monad \Sigma$ there is  a  $\monad$-morphism $				h  : \monad \Sigma \to \alg$
	which recognises $L$ and  factors through  every $\monad$-morphism recognising $L$.

\paragraph*{Terms and polynomials.} For a set of variables $X$, define a \emph{term with variables $X$} to be  an element of $\monad X$. If $\alg$ is a $\monad$-algebra and  $t$ is a term with variables $X$,  and $f : X \to A$ is a valuation of the variables, then define
\begin{align*}
t[v] \eqdef	\mult_\alg (\monad f (t)).
\end{align*}
Define a $\monad$-congruence in a $\monad$-algebra $\alg$ to be a  surjective  function $f : A \to B$  from the universe of $\alg$ to some set $B$ without any further structure, such that $f$  commutes with all terms in the sense that every $w_1,w_2 \in \monad A$ satisfy
	\begin{align*}
		\monad f (w_1) = \monad f (w_2) \qquad \mbox{implies} \qquad f(\mult_\alg (w_1)) = f(\mult_\alg (w_2)).
	\end{align*}
	If this is the case, then one can define, in a unique way, a multiplication operation
	\begin{align*}
		\mult_\balg : \monad B \to B
	\end{align*}
	 which turns  $f$ into a $\monad$-morphism.  In other words, a $\monad$-congruence is a $\monad$-morphism, with the structure of $\monad$-algebra on the image being forgotten.

 An \emph{$n$-ary polynomial} over $\alg$ is a function  $f : A^n \to A$ which is obtained by evaluating some term with $n+k$ variables, under a fixed valuation of the $k$  constants.  

The finiteness assumption of the following lemma is important.
	We say that a function $\tau : X \to X$ preserves a function $\sigma : X \to Y$ if
	\begin{align*}
		\xymatrix { X \ar[r]^\tau \ar[dr]_\sigma & X\ar[d]^\sigma \\ & Y}
	\end{align*}
	commutes.	
	
\begin{lemma}\label{lem:congruence-in-a-finite-algebra}
	Let $\alg$ be a finite algebra.  If  $f : A \to B$ is a surjective function that is preserved by all unary polynomials in $\alg$,  then $f$ is a $\monad$-congruence.
\end{lemma}
\begin{pr}
	We will prove the following claim, where the assumption on finiteness of $A$ is used.
	\begin{claim}
If $g : A \to A$ preserves $f$, then $\monad g$ preserves $f \circ \mult_\alg$.
	\end{claim}
	\begin{pr}
		Suppose that the statement of the lemma holds for two functions $g_1,g_2$. Since functions that preserve $f \circ \mult_\alg$ are closed under composition, and 
		\begin{align*}
			\monad (g_1 \circ g_2) = (\monad g_1) \circ (\monad g_2),
		\end{align*}
		it follows that the statement of the claim also holds for the composition $g_1 \circ g_2$. Therefore it suffices to prove the claim for any set of generators in the monoid of functions $A \to A$ that preserve $f$. By finiteness of $A$,  such a set of generators is the set of functions $g_{ab}$, where   $a,b \in A$, defined by
		\begin{align*}
			g_{ab}(c) = \begin{cases}
				b & \mbox{if $c=a$}\\ a &\mbox{otherwise}.
			\end{cases}
		\end{align*}
		Therefore, we need to prove  that every $w \in \monad A$ satisfies
		\begin{align*}
			f \circ \mult_\alg \circ \monad g_{ab} (w) = f \circ \mult_\alg (w).
		\end{align*}
	The elements $\monad g_{ab} (w)$ and $w$ can be seen as a single term (namely $w$ seen as a term with variables $A$), interpreted under two different valuations that differ only on the variable $a \in A$.  Therefore, the values of $\mult_\alg \circ \monad g_{ab} (w)$ and $\mult_\alg (w)$ are the values of a unary polynomial on arguments $a$ and $b$ respectively. The result follows by the assumption on $f$.
	\end{pr}
	
	Let us now prove the 	statement of the lemma. Let  $w,w' \in \monad A$ be such that $\monad f (w) = \monad f (w')$. By surjectivity of $f$, there is some  $f' : B \to A$ of $f$ such that $g = f' \circ f$ preserves $f$.   The assumption on $w,w'$ implies that
	\begin{align*}
		\monad g (w) = \monad g(w').
	\end{align*}
	The functions $g$ and the identity on $A$ satisfy the assumptions of the claim, and  therefore 
	\begin{align*}
f( \mult_\alg (w)) = 		f(\mult_\alg(\monad g (w))) = f(\mult_\alg(\monad g (w'))) = f(\mult_\alg(w')),
	\end{align*}
	as desired in a $\monad$-congruence. 
\end{pr}

%
% 	% The definition is
% % 	\begin{align*}
% % 		\mult_\calg(w) =  f(\mult_\balg (v)) \qquad \mbox{for some $v \in \monad B$ with $\monad f (v)=w$}
% % 	\end{align*}
% % 	(In the above we assume that if $f$ is surjective, then so is $\monad f$; check if this is always the case.)
% %
%
% Note the dependence on the finiteness assumption in the following lemma.
% 	\begin{claim}\label{claim:commutes-with-unary-polynomials}
% 		Let $\balg$ be a $\monad$-algebra and $f : B \to C$  a function.
% 		\begin{enumerate}
% 			\item  		 If $f$ is a congruence then it commutes with unary polynomials in $\balg$.
% 			\item  If $\balg$ is finite and $f$ commutes with unary polynomials then $f$  is a congruence.
% 		\end{enumerate}
% 	\end{claim}
% 	\begin{pr}
% 		ss
% 	\end{pr}
	
	We now proceed to prove the Myhill-Nerode theorem.
	Define an equivalence relation $\sim$ on $\monad \Sigma$ which identifies two elements 
	$w,v \in \monad \Sigma$ if 
	\begin{align*}
	 f(w) \in L \quad \mbox{iff} \quad f(b) \in L
	\end{align*}
	holds for every unary polynomial $f$ in the algebra $\monad \Sigma$. Define $A$ to be the set of equivalence classes of $\sim$ and let $h : \monad \Sigma \to A$ be the function which maps an element to its equivalence class. Below, we equip $A$ with the structure of a $\monad$-algebra so that $h$ becomes a $\monad$-morphism. Take an arbitrary $\monad$-morphism
	\begin{align*}
		g : \monad \Sigma \to \balg
	\end{align*}
into a finite $\monad$-algebra that recognises $L$, which exists by the assumption that $L$ is $\monad$-recognisable. Because  $g$ recognises $L$, it follows that $g(w)=g(w')$ implies $w \sim w'$. Therefore, there is a unique surjective function $\beta$ that makes the diagram below commute:
	\begin{align*}
		\xymatrix{ \monad \Sigma  \ar[dr]_h \ar[r]^g & \balg \ar[d]^{\beta} \\  & A}
	\end{align*}
One can  check that $\beta$ is preserved by all unary polynomials in $\balg$, and therefore by  Lemma~\ref{lem:congruence-in-a-finite-algebra} it is a congruence. Therefore, one can equip $A$ with the structure of a $\monad$-algebra so that $\beta$ becomes a $\monad$-morphism.

We have shown that for every $h : \monad \Sigma \to \balg$ there is a candidate for the syntactic morphism, namely a $\monad$-morphism 
\begin{align*}
	\beta_h : \monad \Sigma \to \alg_h
\end{align*}
which recognises $L$, has uses an algebra with universe $A$, and factors through $h$. The only problem is that the structure of the algebra $\alg_h$ seems to depend on $h$. To see that there is actually no such dependence, one can apply the construction to a product of morphisms that recognise $L$.
