# Supplementary material for: Recognisable languages over monads
Source: arXiv:1502.04898 source file (2015-02-17)
Supplement: Supplementary file 2 [file appendix-promonad.tex]

\section{Appendix to Section}%~\ref{sec:profinite-monads}}
\label{sec:appendix-profinite-monads}
\subsection{The multiplication  operation in the profinite monad}
In this part of the appendix, we prove Lemma~\ref{lem:pro-multiplication}. The lemma says that for  set $\Sigma$ there exists a unique operation $\overline{\mult}$ which makes the following diagram commute
		\begin{align*}
			\vcenter{\xymatrix @R=2pc
				{ \promonad \promonad \Sigma \ar[d]_{\promonad \bar h}  \ar[rr]^\mult && \promonad \Sigma \ar[d]^{\bar h}\\
				\promonad A \ar[rr]^{\bar \alpha}&  & A
				}}
	\end{align*}
	for every $\monad$-morphism $h : \monad \Sigma \to A$ into a finite $\monad$-algebra $\alpha : \monad A \to A$.

\subsection{The algebraic structure in the profinite monad}
In this part of the appendix, we prove Lemma~\ref{lem:promonad-is-a-monad-algebra}. The lemma says that if $\Sigma$ is a set then:
	\begin{enumerate}
		\item	 $\promonad \Sigma$ becomes a $\monad$-algebra when multiplication is defined by the composition
	\begin{align*}
		\xymatrix@C=4pc{ \monad \promonad \Sigma \ar@{^{(}->}[r] & \promonad \promonad \Sigma \ar[r]^{\mult_{\promonad}} & \promonad \Sigma}.
	\end{align*}
	\item  Let $f : \Sigma \to \Gamma$ be a function. If $\promonad \Sigma$ and $\promonad \Gamma$ are seen as $\monad$-algebras in the sense of item 1, then $\promonad f$
	is a $\monad$-morphism.
\item  If  $\promonad \promonad \Sigma$ and $\promonad \Sigma$ are seen as $\monad$-algebras  in the sense of the item 1, then then $\mult_\promonad$  
	is a $\monad$-morphism.
	\end{enumerate}

	\begin{center}
		(TODO : prove the lemma)
	\end{center}
	
	\begin{align*}
		\vcenter{\xymatrix @R=2pc @C=4pc
			{ \monad \promonad \promonad \Sigma \ar[d]_{ \promonadalg_{\promonad \Sigma}}  \ar[r]^{\monad \mult_{\promonad}} & \monad \promonad \Sigma \ar[d]^{\promonadalg_\Sigma}\\
			 \promonad \promonad \Sigma \ar[r]^{\mult_{\promonad}}  & \promonad
			}}
	\end{align*}
